# Supplementary material for: Translational and rotational dynamics of a self-propelled Janus probe in crowded environments
Source: arXiv:2008.02089 ancillary file (2020-08-05)
Supplement: Supplementary file 1 [file Electronic_Supplementary_Information_14_July_2020.pdf]

# Electronic Supplementary Information: Translational and rotational dynamics of a self-propelled Janus probe in crowded environments

Ligesh Theeyancheri[1], Subhasish Chaki[1], Nairhita Samanta[1], Rohit Goswami[1], Raghunath Chelakkot[2,†] and Rajarshi Chakrabarti[1,*]

1. *Department of Chemistry, Indian Institute of Technology Bombay, Mumbai, Powai 400076, E-mail: rajarshi@chem.iitb.ac.in and*

2. *Department of Physics, Indian Institute of Technology Bombay, Mumbai, Powai 400076, E-mail: raghu@phy.iitb.ac.in*

(Dated: August 5, 2020)

The method of validation is performed for a self-propelled free Janus probe. The translational mean square displacement ($\langle \Delta r_c^2(\tau)\rangle$) and rotational mean square displacement ($\langle \Delta\theta^2(\tau)\rangle$) are calculated as follows:

$$\left\langle \Delta r_c^2(\tau)\right\rangle = \left\langle \overline{\left[r_c\Big(t+\tau\Big) - r_c\Big(t\Big)\right]^2}\right\rangle \tag{1}$$

$$\left\langle \Delta\theta^2(\tau)\right\rangle = \left\langle \overline{\left[\theta\Big(t+\tau\Big) - \theta\Big(t\Big)\right]^2}\right\rangle \tag{2}$$

From the plot for $F = 0$ (Fig. 2(b) in the manuscript), we have calculated $D_T = 0.03266$ and $\xi = \frac{k_B T}{D_T} = 30.61$. The rotational diffusivity ($D_R$) is calculated from $\langle \Delta\theta^2(\tau)\rangle$ plot (Fig. 3(b) in the manuscript). Hence, $\tau_R = \frac{1}{D_R} = 2.63 \times 10^{-3}$. Using the values of $D_T$ and $\tau_R$, $\langle \Delta r_c^2(\tau)\rangle$ is fitted with the analytical expression:

$$\left\langle \Delta r_c^2(\tau)\right\rangle = \left[4D_T + 2v^2\tau_R\right]\tau + 2v^2\tau_R^2\left[e^{-\frac{\tau}{\tau_R}} - 1\right] \tag{3}$$

where $v = \frac{F}{\xi}$.

The velocity autocorrelation function ($C_{\mathrm{v}}(\tau)$) is calculated for the passive and the Janus probe subjected to different self-propulsion as follows:

$$C_{\mathrm{v}}(\tau) = \frac{\left\langle \overline{\mathbf{v}(t+\tau).\mathbf{v}(t)}\right\rangle}{\left\langle \overline{v^2(t)}\right\rangle} \tag{4}$$

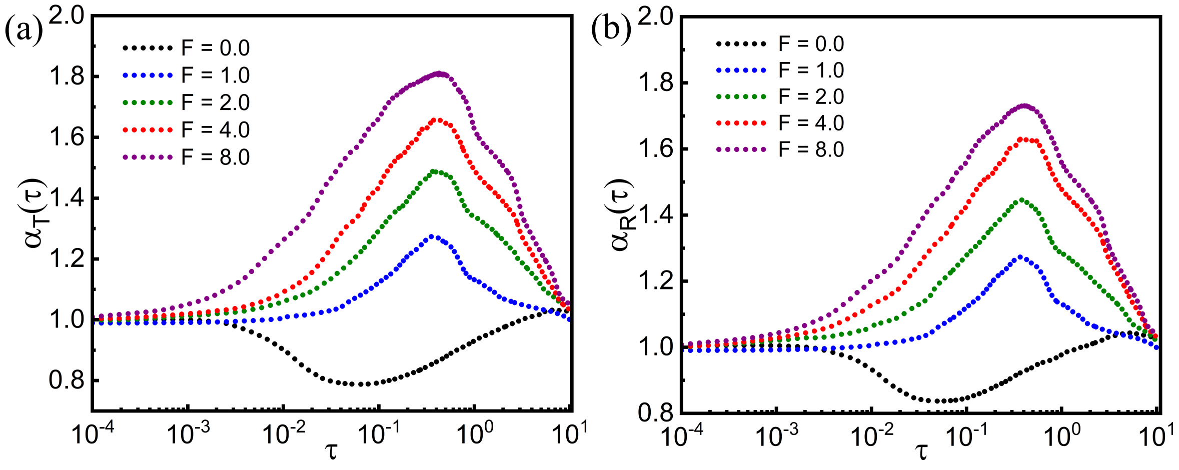


FIG. 1: The time exponents (a) $\alpha_T(\tau)$ and (b) $\alpha_R(\tau)$ for the passive and self-propelled Janus probe with different self-propulsion $F$ in purely repulsive polymers ($\phi = 0.165$).

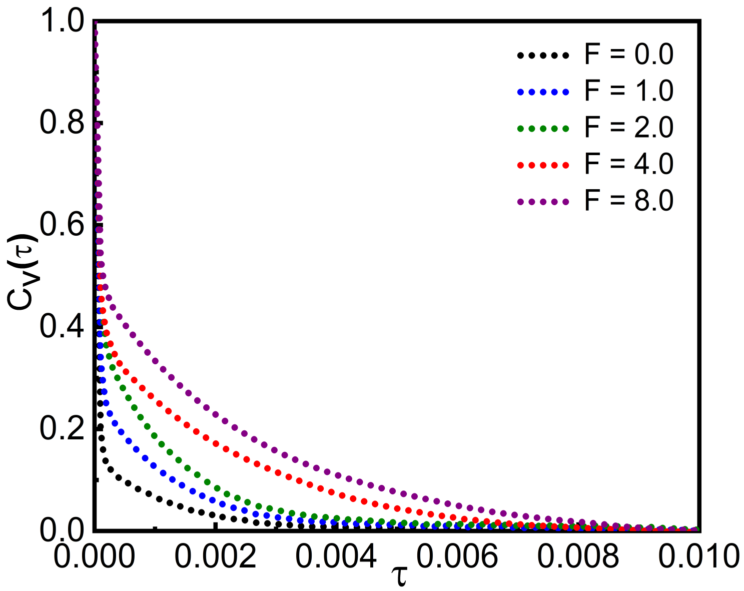


FIG. 2: $C_{\mathrm{v}}(\tau)$ *vs* $\tau$ for the passive and self-propelled Janus probe with different self-propulsion $F$ in purely repulsive polymers ($\phi = 0.165$).

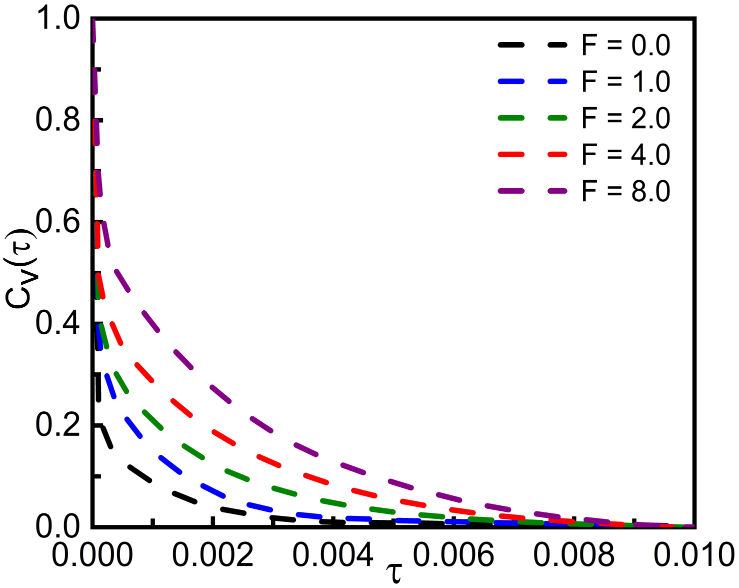


FIG. 3: $C_{\rm v}(\tau)$ *vs* $\tau$ for the passive and self-propelled Janus probe with different self-propulsion $F$ in purely repulsive colloidal particles ($\phi = 0.165$).

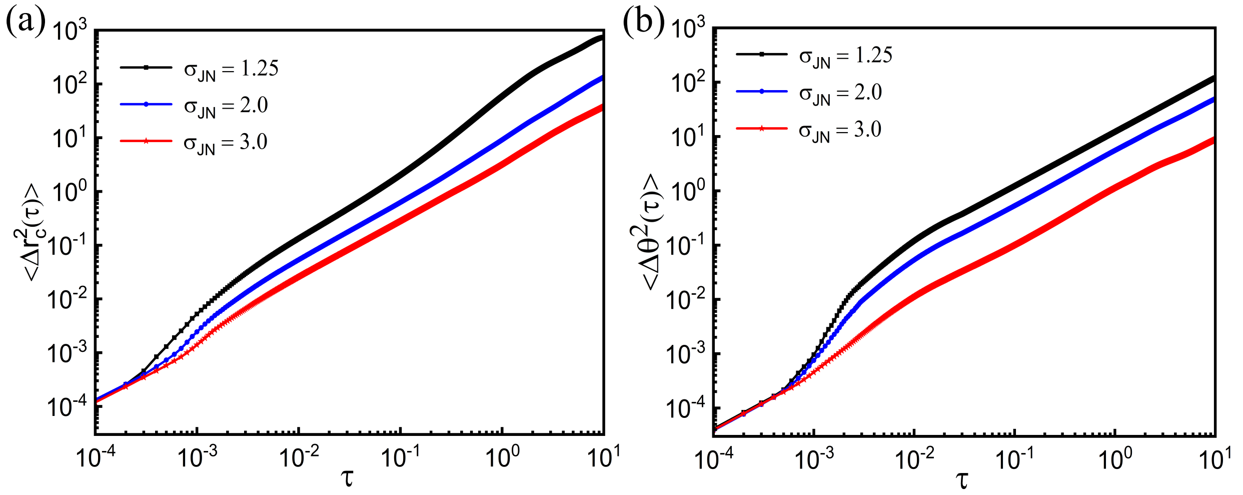


FIG. 4: Log-Log plot of (a) $\langle \Delta r_c^2(\tau)\rangle$ *vs* $\tau$ and (b) $\langle \Delta\theta^2(\tau)\rangle$ *vs* $\tau$ for the self-propelled Janus probe subjected to $F = 8.0$ in polymers with sticky zone ($\epsilon = 2.0$) for $\phi = 0.165$.

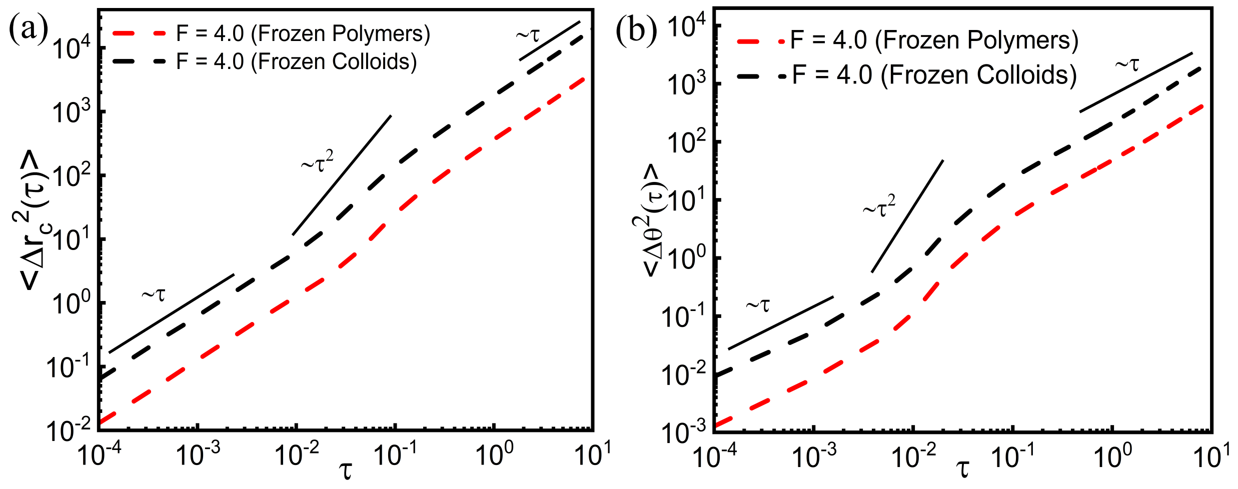


FIG. 5: Log-Log plot of (a) $\langle \Delta r_c^2(\tau) \rangle$ $vs$ $\tau$ and (b) $\langle \Delta\theta^2(\tau) \rangle$ $vs$ $\tau$ for the self-propelled Janus probe subjected to $F = 4.0$ in purely repulsive frozen colloids and frozen polymers ($\phi = 0.165$).

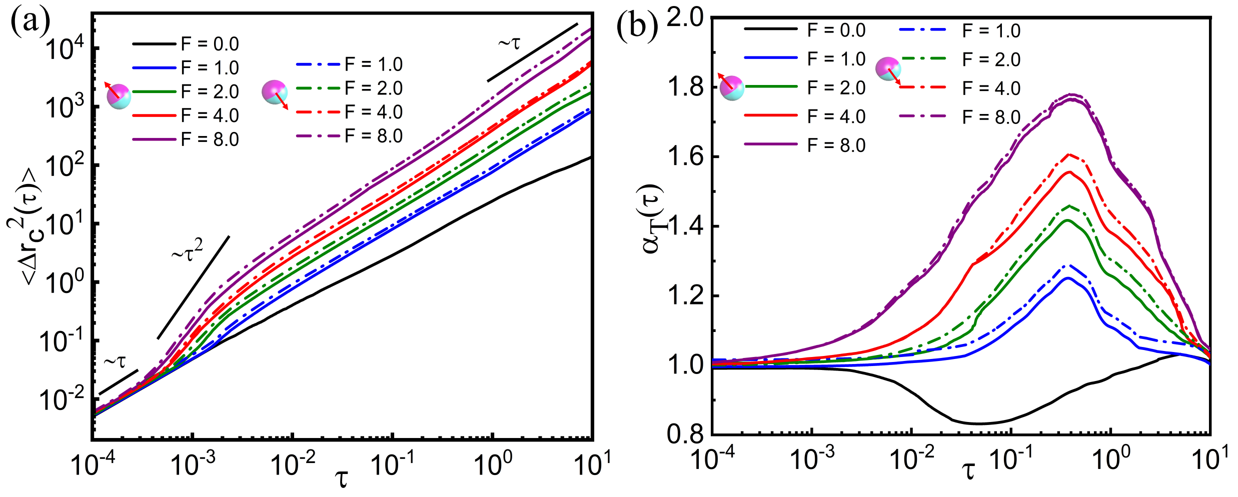


FIG. 6: Log-Log plot of (a) $\langle \Delta r_c^2(\tau) \rangle$ $vs$ $\tau$ for the passive and self-propelled Janus probe subjected to different $F$ in a binary mixture of attractive ($\epsilon = 2.0$) and repulsive colloids with self-propulsion towards sticky (solid lines), non-sticky face (dash-dotted lines) for $\phi = 0.165$ and (b) The corresponding exponents $\alpha_T(\tau)$.

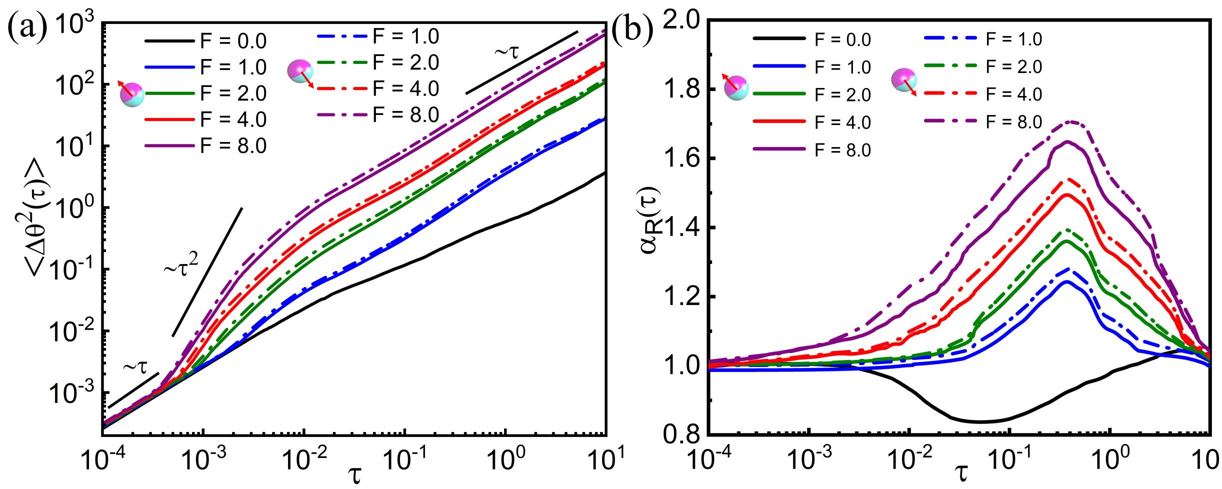


FIG. 7: Log-Log plot of (a) $\langle\Delta\theta^2(\tau)\rangle$ $vs$ $\tau$ for the passive and self-propelled Janus probe subjected to different $F$ in a binary mixture of attractive ($\epsilon = 2.0$) and repulsive colloids with self-propulsion towards sticky (solid lines), non-sticky face (dash-dotted lines) for $\phi = 0.165$ and (b) the corresponding exponents $\alpha_R(\tau)$.

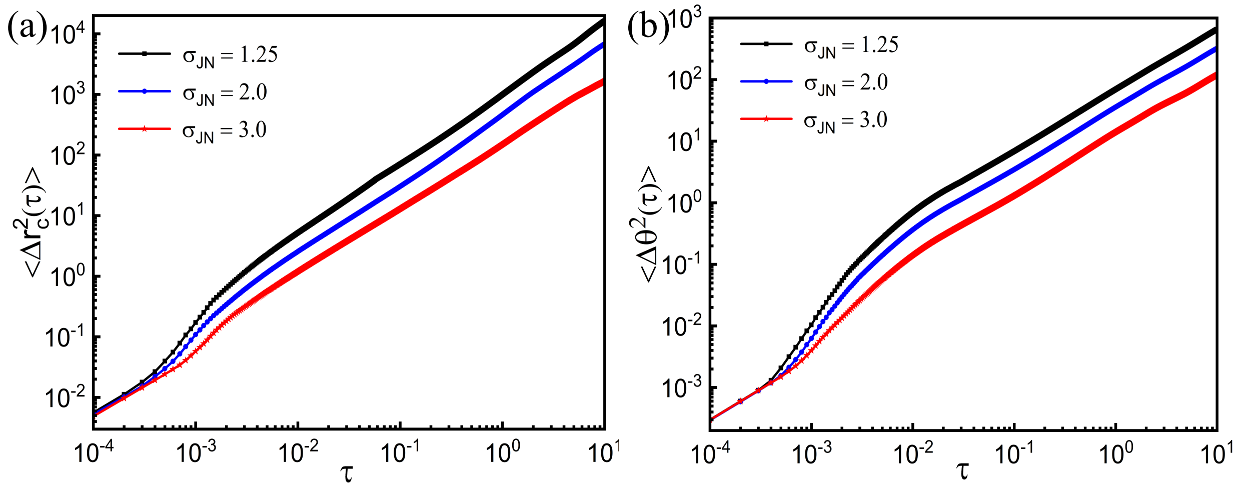


FIG. 8: Log-Log plot of (a) $\langle\Delta r_c^2(\tau)\rangle$ $vs$ $\tau$ and (b) $\langle\Delta\theta^2(\tau)\rangle$ $vs$ $\tau$ for the self-propelled Janus probe subjected to $F = 8.0$ in a binary mixture of attractive ($\epsilon = 2.0$) and repulsive colloids ($\phi = 0.165$).

### A. Mean square displacements of a self-propelled Janus probe in different area fractions ($\phi$) of the medium

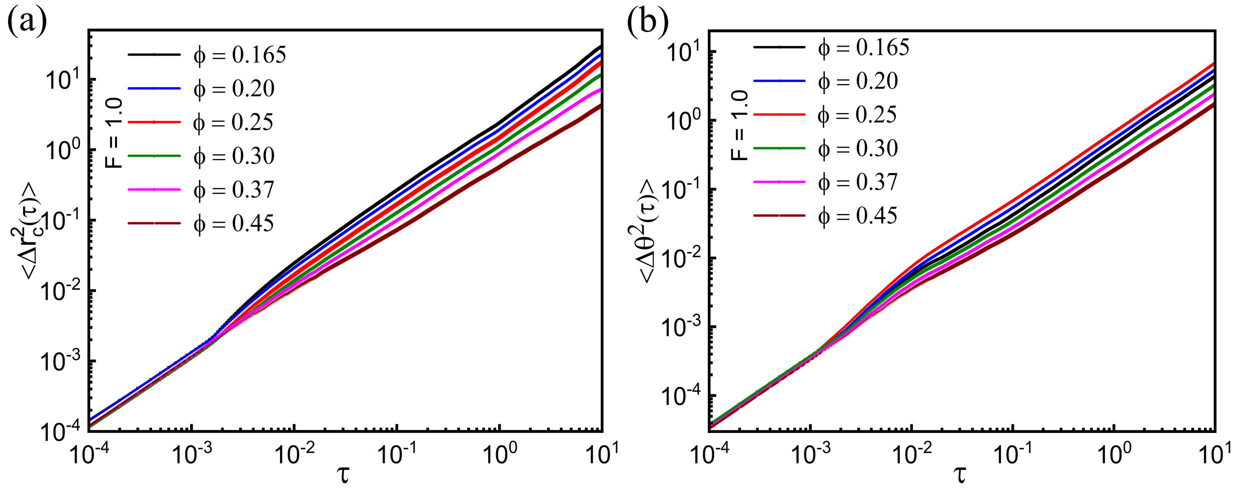


FIG. 9: Log-Log plot of (a) $\langle \Delta r_c^2(\tau) \rangle$ $vs$ $\tau$ and (b) $\langle \Delta\theta^2(\tau) \rangle$ $vs$ $\tau$ for the self-propelled Janus probe in different area fractions of polymer with sticky zones ($\epsilon = 2.0$) for $F = 1.0$. The black dashed lines represents the best possible fit of Eq. 6.

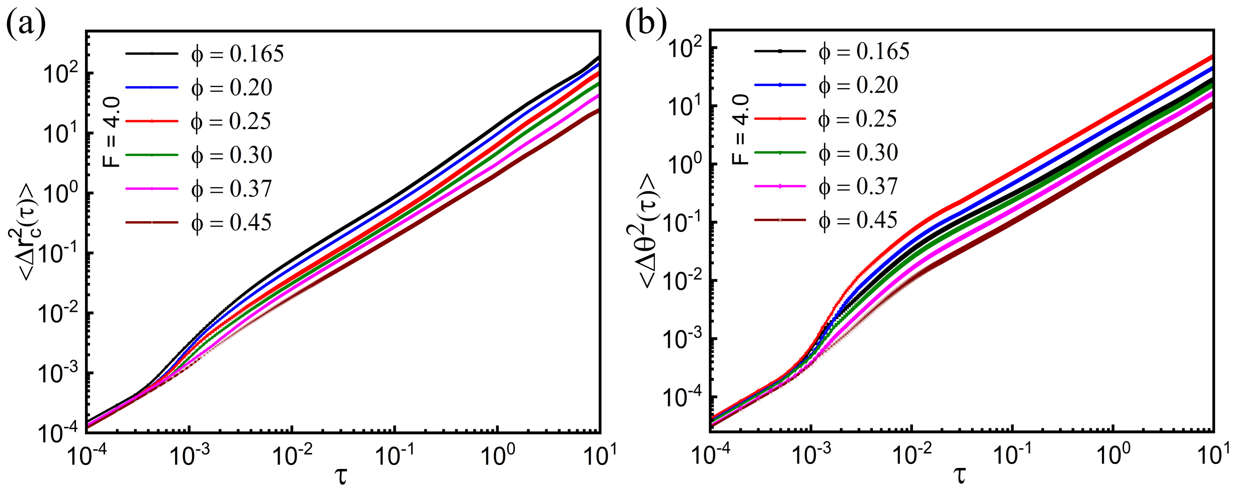


FIG. 10: Log-Log plot of (a) $\langle \Delta r_c^2(\tau) \rangle$ $vs$ $\tau$ and (b) $\langle \Delta\theta^2(\tau) \rangle$ $vs$ $\tau$ for the self-propelled Janus probe in different area fractions of polymer with sticky zones ($\epsilon = 2.0$) for $F = 4.0$. The black dashed lines represents the best possible fit of Eq. 6.

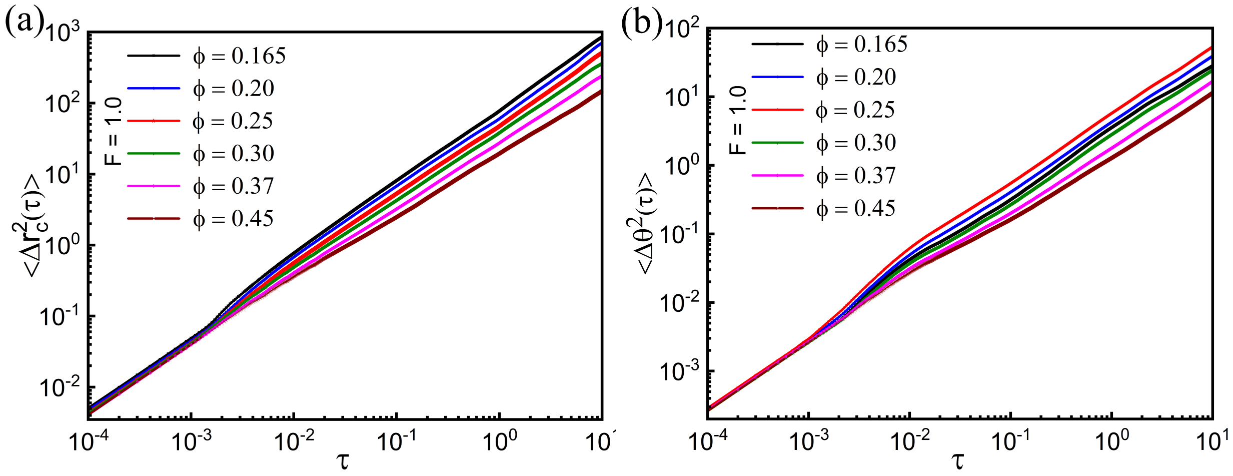


FIG. 11: Log-Log plot of (a) $\langle \Delta r_c^2(\tau) \rangle$ $vs$ $\tau$ and (b) $\langle \Delta\theta^2(\tau) \rangle$ $vs$ $\tau$ for the self-propelled Janus probe in different area fractions of a binary mixture of attractive ($\epsilon = 2.0$) and repulsive colloids for $F = 1.0$. The black dashed lines represents the best possible fit of Eq. 6.

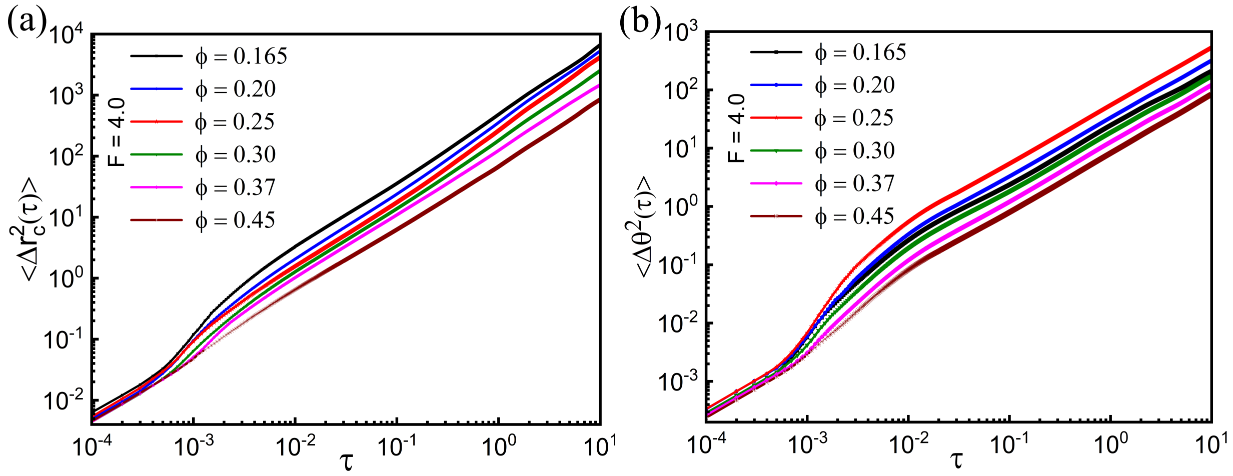


FIG. 12: Log-Log plot of (a) $\langle \Delta r_c^2(\tau) \rangle$ $vs$ $\tau$ and (b) $\langle \Delta\theta^2(\tau) \rangle$ $vs$ $\tau$ for the self-propelled Janus probe in different area fractions of a binary mixture of attractive ($\epsilon = 2.0$) and repulsive colloids for $F = 4.0$. The black dashed lines represents the best possible fit of Eq. 6.

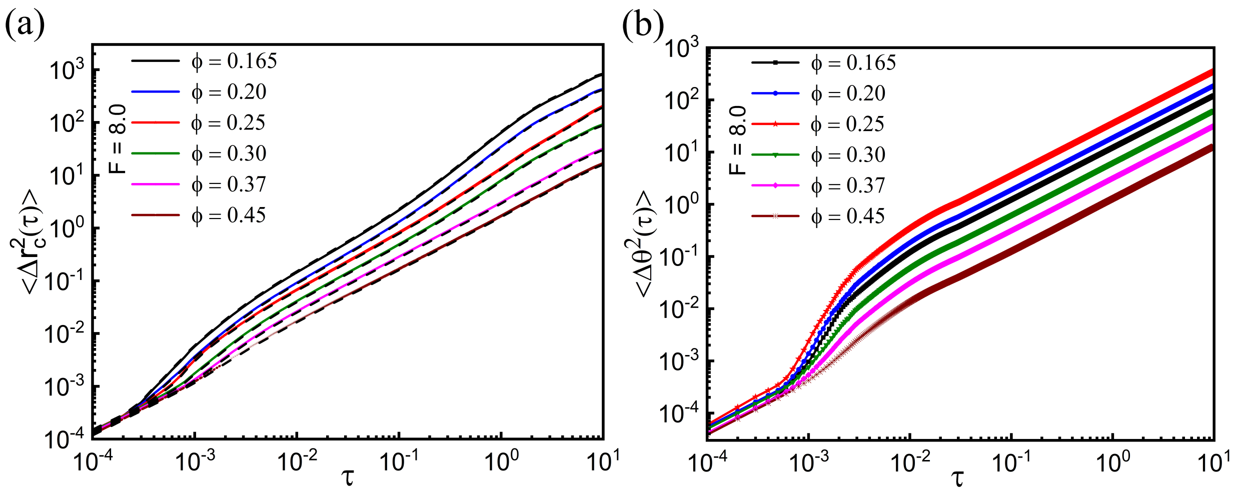


FIG. 13: Log-Log plot of (a) $\langle \Delta r_c^2(\tau) \rangle$ $vs$ $\tau$ and (b) $\langle \Delta\theta^2(\tau) \rangle$ $vs$ $\tau$ for the self-propelled Janus probe in different area fractions of polymer with sticky zones ($\epsilon = 2.0$) for $F = 8.0$. The black dashed lines represents the best possible fit of Eq. 6.

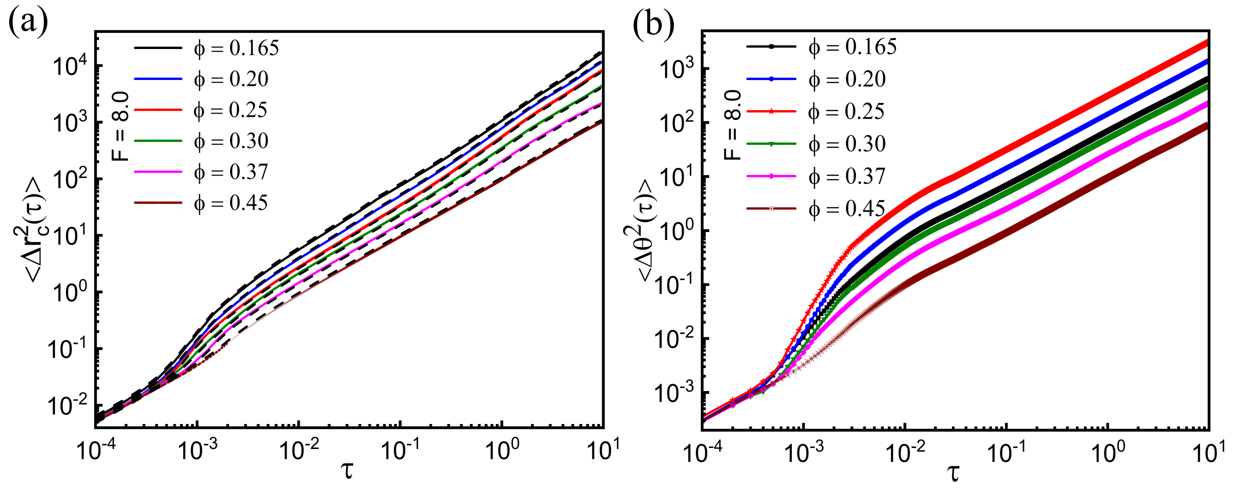


FIG. 14: Log-Log plot of (a) $\langle \Delta r_c^2(\tau) \rangle$ $vs$ $\tau$ and (b) $\langle \Delta\theta^2(\tau) \rangle$ $vs$ $\tau$ for the self-propelled Janus probe in different area fractions of a binary mixture of attractive ($\epsilon = 2.0$) and repulsive colloids for $F = 8.0$. The black dashed lines represents the best possible fit of Eq. 6.

| $\phi$ | Polymers | | Colloids | |
|---|---|---|---|---|
| | $v$ | $\tau_R$ | $v$ | $\tau_R$ |
| 0.165 | 0.2587 | $2.935 \times 10^{-3}$ | 0.2604 | $2.8247 \times 10^{-3}$ |
| 0.20 | 0.2502 | $2.9142 \times 10^{-3}$ | 0.2568 | $2.7985 \times 10^{-3}$ |
| 0.25 | 0.2476 | $2.8945 \times 10^{-3}$ | 0.2495 | $2.7046 \times 10^{-3}$ |
| 0.30 | 0.2351 | $2.9182 \times 10^{-3}$ | 0.2386 | $2.8095 \times 10^{-3}$ |
| 0.37 | 0.2205 | $2.926 \times 10^{-3}$ | 0.2241 | $2.8347 \times 10^{-3}$ |
| 0.45 | 0.2115 | $2.9613 \times 10^{-3}$ | 0.2145 | $2.8845 \times 10^{-3}$ |

TABLE I: The $\left\langle \Delta r_c^2(\tau) \right\rangle$ fitting parameters, $v$ and $\tau_R$ for different area fractions $\phi$ of the self-propelled Janus probe in polymers having sticky zones (Fig. 13(a)) and binary mixture of stciky and non-sticky colloids (Fig. 14(a)) for $F = 8.0$.

### B. Mean square displacements and velocity autocorrelation of a self-propelled Janus probe with higher binding affinity ($\epsilon = 4.0$) for $\phi = 0.165$

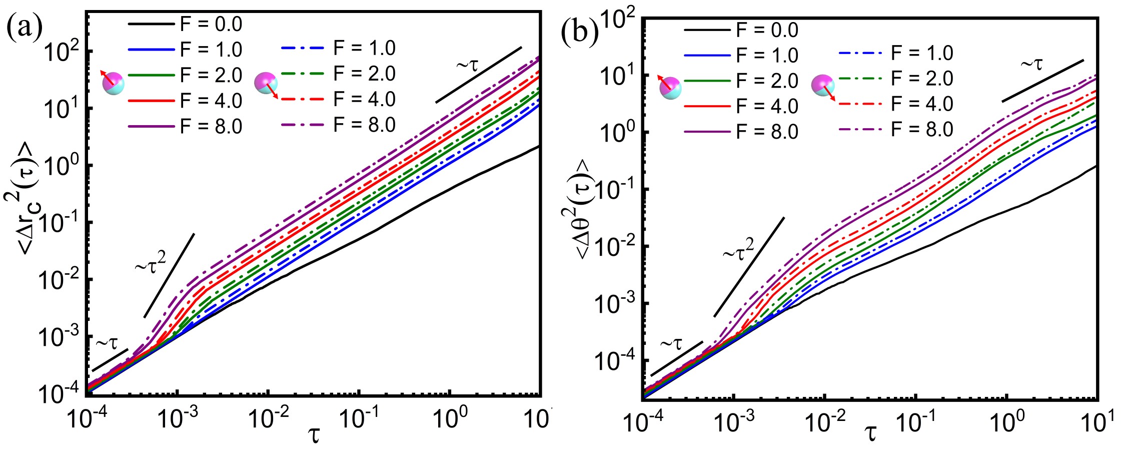


FIG. 15: Log-Log plot of (a) $\langle \Delta r_c^2(\tau) \rangle$ *vs* $\tau$ for the passive and self-propelled Janus probe subjected to different $F$ in polymers with sticky zones ($\epsilon = 4.0$) and (b) $\langle \Delta\theta^2(\tau) \rangle$ *vs* $\tau$ for the same. In both cases the solid lines, dash-dotted lines represent the self-propulsion towards sticky face and the non-sticky face of the Janus probe respectively.

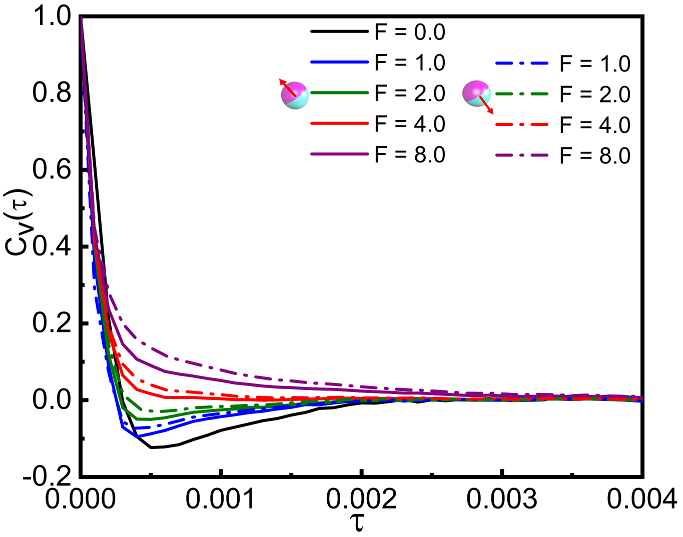


FIG. 16: Log-Log plot of $C_{\rm v}(\tau)$ *vs* $\tau$ for the passive and self-propelled Janus probe subjected to different $F$ in polymers with sticky zones ($\epsilon = 4.0$) with self-propulsion towards sticky face (solid lines) and the non-sticky face (dash-dotted lines) of the Janus probe.

**Movies**

The movies illustrate the qualitative difference in the dynamics of the self-propelled Janus probe in crowded heterogeneous environments. In all the cases, only the magenta part of the Janus probe is attractive to the blue monomers and remaining all interactions are purely repulsive.

1. Movie-1_PolymerJanus_Passive.mp4

   Molecular dynamics simulation of passive Janus probe in a sea of polymers having attractive zones (blue monomers) with $\epsilon = 2$. The Janus probe get confined inside a cavity created by the polymers and then as the time progresses, it escapes from the cavity.

2. Movie-2_PolymerJanus_Self-propulsion_Sticky.mp4

   Molecular dynamics simulation of self-propelled Janus probe with $F = 8.0$ directed towards the sticky face of the Janus probe in a sea of polymers having attractive zones (blue monomers) for $\epsilon = 2$. The Janus shows some tendency to stick to the attractive part of the polymer for a while and the moves apart.

3. Movie-3_PolymerJanus_Self-propulsion_Non-sticky.mp4

   Molecular dynamics simulation of self-propelled Janus probe with $F = 8.0$ directed towards the non-sticky face of the Janus probe in a sea of polymers having attractive zones (blue monomers) for $\epsilon = 2$. The direction of self-propulsion helps the Janus probe to escapes from the attractive part of the polymers.

4. Movie-4_ColloidsJanus_Self-propulsion.mp4

   Molecular dynamics simulation of self-propelled ($F = 8.0$) Janus probe in a binary mixture of attractive ($\epsilon = 2$) and repulsive colloids. There is no confinement due to cavity, and the Janus probe frequently encounter the colloids and perform faster rotation and translation.

5. Movie-5_Frozen_PolymerJanus_WCA.mp4

   Molecular dynamics simulation of self-propelled Janus probe with $F = 4.0$ in a sea of

purely repulsive frozen polymers. The Janus probe feels a prolonged confinement due to the surrounding rigid polymers.

6. Movie-6_Frozen_ColloidsJanus_WCA.mp4
   Molecular dynamics simulation of self-propelled Janus probe with $F = 4.0$ in a sea of purely repulsive frozen colloids. There is no confined motion as one can see in frozen polymers.
